# Supplementary material for: Hierarchical Planning for Dynamic Resource Allocation in Smart and Connected Communities
Source: arXiv:2107.01292 source file (2021-12-20)
Supplement: Supplementary file 1 [file appendix.tex]

%------------------------------------------------
% Appendix
%------------------------------------------------

\newpage
% \newpage
\appendix
\appendixpage

\section{Simulator}
\label{sec:app_sim}

This appendix describes our simulation of the emergency response system and the environment used by the low-level planner to estimate the effect of various actions. As shown in figure \ref{fig:state}, our system state at time $t$ is captured by a queue of active incidents $I^{t}$ and agent states $\Lambda$. $I^t$ is the queue of incidents that have been reported but not yet serviced, and allows the system to keep track of any incidents that could not be immediately responded to. The state of each agent $\lambda_j \in \Lambda$ consists of the agent's current location $p_j^t$, status $u_j^t$ destination $g_j^t$, assigned region $r_j^t$, and assigned depot $d_j^t$. Each agent can be in several different internal states (represented by $u_j^t$), including \textit{waiting} (waiting at a depot), \textit{in\_transit} (moving to a new depot and not in emergency response mode), \textit{responding} (the agent has been dispatched to an incident and is moving to its location), and \textit{servicing} (the agent is currently servicing an incident). These states dictate how the agent is updated when moving the simulator forward in time. 

To determine the travel times between locations in the environment, the simulator uses a traffic router. In our experiments, we use a Euclidean distance based router, which assumes all agents travel in straight lines between locations. If deployed to a real world system, a more advanced router can be used that uses information about the roadway network and current traffic conditions to accurately estimate travel times. 

Our simulator is designed as a discrete event simulator, meaning that the state is only updated at discrete time steps when interesting events occur. These events include incident occurrence, re-allocation planning steps, and responders becoming available for dispatch. Between these events, the system evolves based on prescribed rules. Using a discrete event simulator saves on valuable computation time as compared to a continuous time simulator. 

At each time step when the simulator is called, the system's state is updated to the current time of interest. First, if the current event of interest is an incident occurrence, it is added to the active incidents queue $I^t$. Then each agent's state and locations are updated to where they would be at the given time, which depends on their current state. For example, agents that are in the \textit{waiting} state stay at the same position, while agents that are \textit{responding} or \textit{in\_transit} will check to see if they have reached their destination. If they have, they will update their state to \textit{servicing} or \textit{waiting} respectively and update their locations. If they have not reached their destination, they interpolate their current location using the travel model. If an agent is in the \textit{servicing} state and finishes servicing an incident, it will enter the \textit{in\_transit} state and set its destination $g_j^t$ to its assigned depot. 

After the state is updated, a planner has several actuation's available to control the system. The \textit{Dispatch}$(\lambda_j, \textit{incident})$ function will dispatch the agent $\lambda_j$ to the given incident which is in $I^t$. Assuming the responder is available, the system sets $\lambda_j$'s destination $g_j^t$ to the incident's location, and its status $u_j^t$ is set to \textit{responding}. The incident is also removed from $I^t$ since it is being serviced, and the response time is returned to the planner for evaluation. The planner can also change the allocation of the agents.

\textit{AssignRegion}$(\lambda_j, r_j)$ assigns agent $\lambda_j$ to region $r_j$ by updating $\lambda_j$'s $r_j^t$. \textit{AssignDepot}$(\lambda_j, d_j)$ similarly assigns agent $\lambda_j$ to depot $d_j$ by updating $\lambda_j$'s $d_j^t$ and setting its destination $g_j^t$ to the depots location. These functions allow a planner to try different allocations and simulate various dispatching decisions. 

\section{Notation}

We summarize notation in table \ref{tab:lookup-table}.  

\input{notations}

\section{Reproducibility}

We have made the code used in this study publicly available.\footnote{\href{https://github.com/StatResp/Hierarchical_ERM_ICCPS}{https://github.com/StatResp/Hierarchical\_ERM\_ICCPS}} Detailed instructions on how to use the code can be found in the repository's readme. Below is an overview of the code and where to find various components.

\begin{itemize}
    \item \textbf{Decision\_making}: This folder contains the bulk of the decision process's implementation. \textit{MMCHighLevelPolicy.py} implements the high level planner. The \textit{./LowLevel/} folder contains the low level policy implementation, including the MCTS implementation, the reward function, and more. The \textit{./coordinator/} folder contains the various decision coordinator implementations, which control what decision strategy is used. For example, \textit{DispatchOnlyCoord.py} implements a static allocation policy. 
    
    \item \textbf{Environment}: This folder contains the simulator and information about the problem's environment. For example, \textit{ResponderDynamics.py} defines responders' behavior,  \textit{CellTravelModel.py} defines how long it takes to travel between locations, and \textit{Spatial/spatialStructure.py} defines the spatial grid which discretizes the environment.
    
    \item \textbf{Prediction}: This folder contains the incident forecasting model. 
    
    \item \textbf{Scenarios}: This folder contains definitions of different experimental scenarios that can be run. This includes defining the experimental environment, setting up the decision framework, and running the experiment. For example, \textit{./gridworld\_example/} defines a simple gridworld environment for demonstration purposes. 
    
\end{itemize}

To run an experiment, go to the appropriate scenario folder and run the experiment's script. This will define the environment, load the appropriate forecasting model, construct the desired decision framework, and then run a simulated ERM system using the desired allocation strategy. More information for how the framework is configured and how to define your own experiment can be found in the repository's readme. 

The incident data used in this study is proprietary, but we have released a synthesized example dataset (in the \textit{data/} folder) to demonstrate the expected data format. The incident data consists of a time series of incident events, each of which has a location and time of occurrence. We have provided a chain of synthetic `real incidents', which are used to evaluate the model, as well as several chains of incidents sampled from the forecasting model which are used in planning. We have run example experiments on this synthetic data, which are defined in the \textit{scenarios/synthesized/} folder, and have provided our results for reference.
